# Supplementary material for: Smallest Fullerene-like Structures of Boron with Cr, Mo, and W Encapsulation
Source: arXiv:1907.12611 source file (2019-07-29)
Supplement: Supplementary file 1 [file Supplementary-Information.pdf]

# Smallest Fullerene-like Structures of Boron with Cr, Mo, and W Encapsulation

Amol B. Rahane[1,2], Pinaki Saha[3], N. Sukumar[3,4] and Vijay Kumar[1,4]

[1]Dr. Vijay Kumar Foundation, 1969, Sector 4, Gurgaon - 122 001, Haryana, India.

[2]Department of Physics, K. R. T. Arts, B. H. Commerce and A. M. Science (KTHM) College, Nashik - 422 002, Maharashtra, India.

[3]Department of Chemistry, School of Natural Sciences, Shiv Nadar University, NH-91, Tehsil Dadri, Gautam Buddha Nagar 201314, Uttar Pradesh, India.

[4]Center for Informatics, School of Natural Sciences, Shiv Nadar University, NH-91, Tehsil Dadri, Gautam Buddha Nagar 201314, Uttar Pradesh, India.

## Supplementary Information

We have performed calculations on neutral, cation, and anion clusters using Gaussian09 program with B3PW91 and PBE0 hybrid exchange-correlation functionals. For Cr encapsulation, we used 6-311+G basis set, whereas for Mo and W encapsulation LANL2DZ basis set has been used.

Figure S1 shows the low-lying isomers for neutral $MB_{18}$ (M = Cr, Mo, and W). In all cases the lowest energy isomer with Gaussian09 calculations remains similar to that in VASP calculations. For the $CrB_{18}$ cluster the capped drum structure having $B_{16}$ double ring tubular (DRT) structure and two boron capping on one side (isomer I in Fig. S1) is the lowest in energy, whereas isomers II and III are, respectively, 1.15 eV and 1.45 eV higher in energy than isomer I. Isomer II is a drum-like structure with metal atom at the center of the $B_{18}$ DRT structure, which is the lowest in energy for $MoB_{18}$ and $WB_{18}$. For $MoB_{18}$ and $WB_{18}$ isomer I is, respectively, 0.36 eV and 0.42 eV higher in energy than isomer II. Some of the low-lying isomers for neutral $M@B_{20}$ (M = Cr, Mo, and W) are shown in Fig. S2. For $Cr@B_{20}$, isomer I has the lowest energy, whereas several isomers (II to XII) are nearly degenerate (within 0.05-0.35 eV) with isomer I. For $Mo@B_{20}$ and $W@B_{20}$ isomer XII has the lowest energy while isomer I is 1.79 eV and 2.06 eV higher in energy than isomer XII for Mo and W cases, respectively. Figures S3 and S4 show some of the low-lying isomers of neutral $M@B_{22}$ and $M@B_{24}$ (M = Cr, Mo, and W). For $Cr@B_{22}$ isomer I with $D_2$ symmetry in Fig S3 is the lowest in VASP-PBE calculations and Gaussian09 B3PW91 calculations. However, using the PBE0 functional in Gaussian09 code, isomer III (a slightly changed $C_1$ symmetry cage) becomes lowest in energy and isomer I is 0.36 eV higher than isomer III. For Mo and W encapsulated $B_{22}$ and Cr, Mo

and W encapsulated $B_{24}$ cages the lowest energy isomers remain similar to those in the VASP calculations.

For the cation cases, the order of isomers remains the same for Cr, Mo and W doped $B_{18}$ as that of the respective neutral structures. For $Cr@B_{18}^{+}$ the bicapped structure (isomer I) is of the lowest energy and the drum structure (isomer II) is 1.03 eV higher in energy than isomer I. For $Mo@B_{18}^{+}$ and $W@B_{18}^{+}$ the bicapped structure (isomers I) is 0.64 eV and 0.59 eV, respectively, higher in energy than isomer II. For $Cr@B_{18}^{-}$ anion the bicapped structure (isomer I) has the lowest energy and drum structure (isomer II) is 0.92 eV higher in energy using Gaussian09 at the PBE0 level. For $Mo@B_{18}^{-}$ and $W@B_{18}^{-}$ the drum structure (isomer II) has the lowest energy and the bicapped structure (isomer I) lies 1.30 eV and 1.21 eV, respectively higher in energy than isomer II. For Cr encapsulation of the cation $B_{20}$ cage, the order of the isomers I and XII swaps compared with the neutral case. Isomer XII has lower energy and isomer I lies 0.38 eV higher. Moreover, the lowest energy isomer of the cation of $Cr@B_{20}$ has been obtained from $W@B_{20}$ which transforms to a cage with an octagon, a heptagon, and two hexagons. It is 0.143 eV lower in energy than isomer XII. On the other hand, for $Mo@B_{20}^{+}$ ($W@B_{20}^{+}$) isomer XII remains the lowest in energy as in the neutral case and isomer I lies 2.80 eV (2.93 eV) higher in energy. However, a cage isomer of $Mo@B_{20}$ ($W@B_{20}$) derived from the cation of $Cr@B_{20}$ lies only 0.686 eV (0.171 eV) higher in energy than isomer XII. For $Cr@B_{20}^{-}$ isomer I has the lowest energy, whereas isomer XII is 0.26 eV higher in energy than isomer I. On the other hand, for $Mo@B_{20}^{-}$ and $W@B_{20}^{-}$ the bicapped drum structure (isomer XII) is 1.03 eV and 1.36 eV lower in energy than the cage structure (isomer I), respectively. However, another cage isomer of anion $Mo@B_{20}$ ($W@B_{20}$) has the lowest energy and it lies 0.202 eV (0.196 eV) lower in energy than the one obtained from isomer XII. Similar to the cation, it has an octagon, a heptagon, and two hexagons. For $Cr@B_{22}^{+}$ isomer III is lower in energy as in the case of neutral (PBE0 level) while isomer I lies 0.90 eV higher. For the cation case of Mo and W encapsulation in $B_{22}$ case, the order of isomers III and I changes. For $Mo@B_{22}^{+}$ ($W@B_{22}^{+}$) isomer III is 0.54 eV (0.33 eV) lower in energy than isomer I. The order of the isomers remains similar for the cation cases of Cr, Mo and W encapsulated $B_{24}$ as for the neutral. For the anion case of Cr encapsulation in $B_{22}$ cage, isomer III has at the lowest energy and isomer I is 0.23 eV higher than isomer III. For anion of Mo encapsulated $B_{22}$, isomer III is 0.064 eV higher in energy than isomer I while for $W@B_{22}$ anion obtained from isomer III is 1.03 eV higher than the one obtained from isomer I. For the metal encapsulated $B_{24}$ anion the order of isomers remains the same as that of the neutral case.

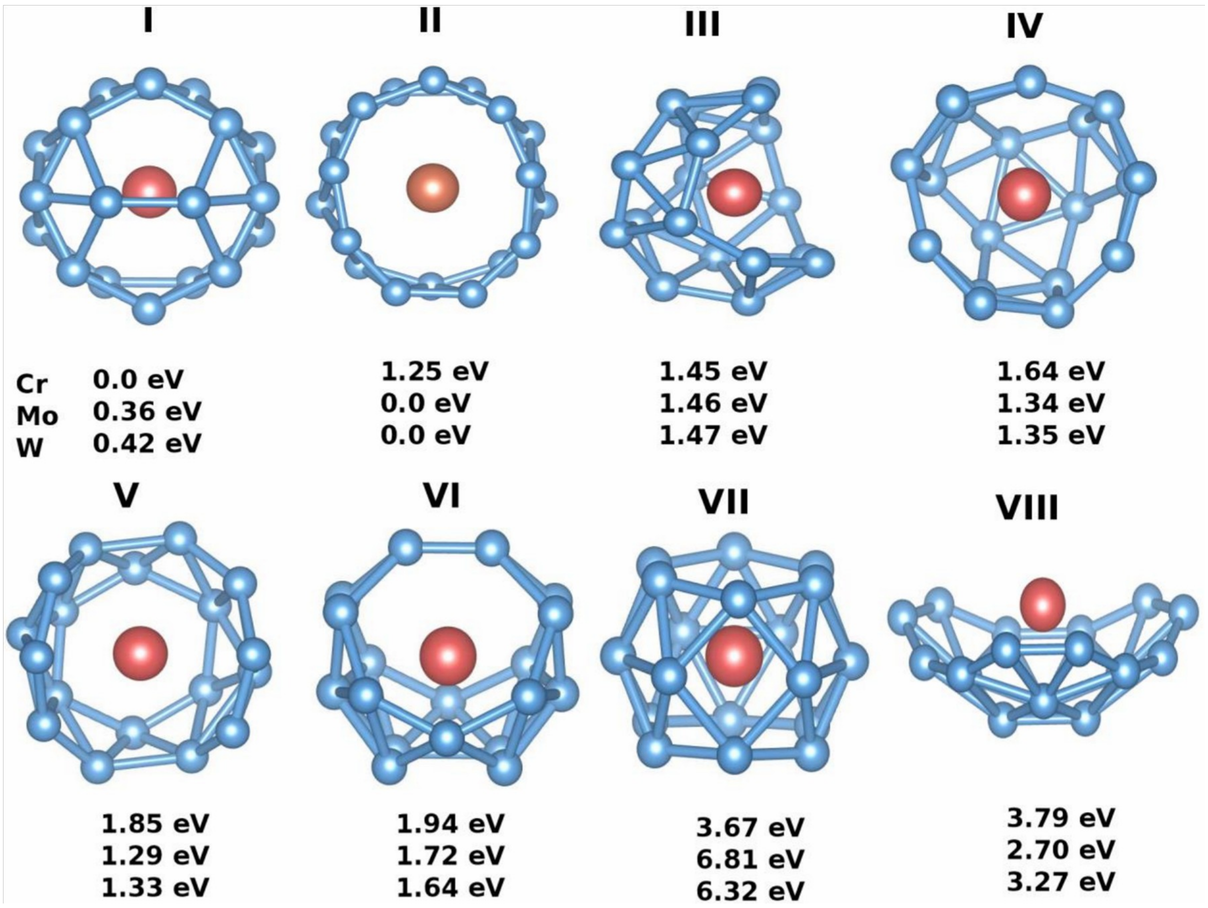


Fig. S1. Some of the low-lying isomers of neutral M@$B_{18}$ (M = Cr, Mo, and W) obtained from VASP calculations using PBE. For each M the energies of different isomers are given with respect to the energy of the lowest energy isomer which has been taken as reference. Blue (red) balls show B (metal) atoms in all structures.

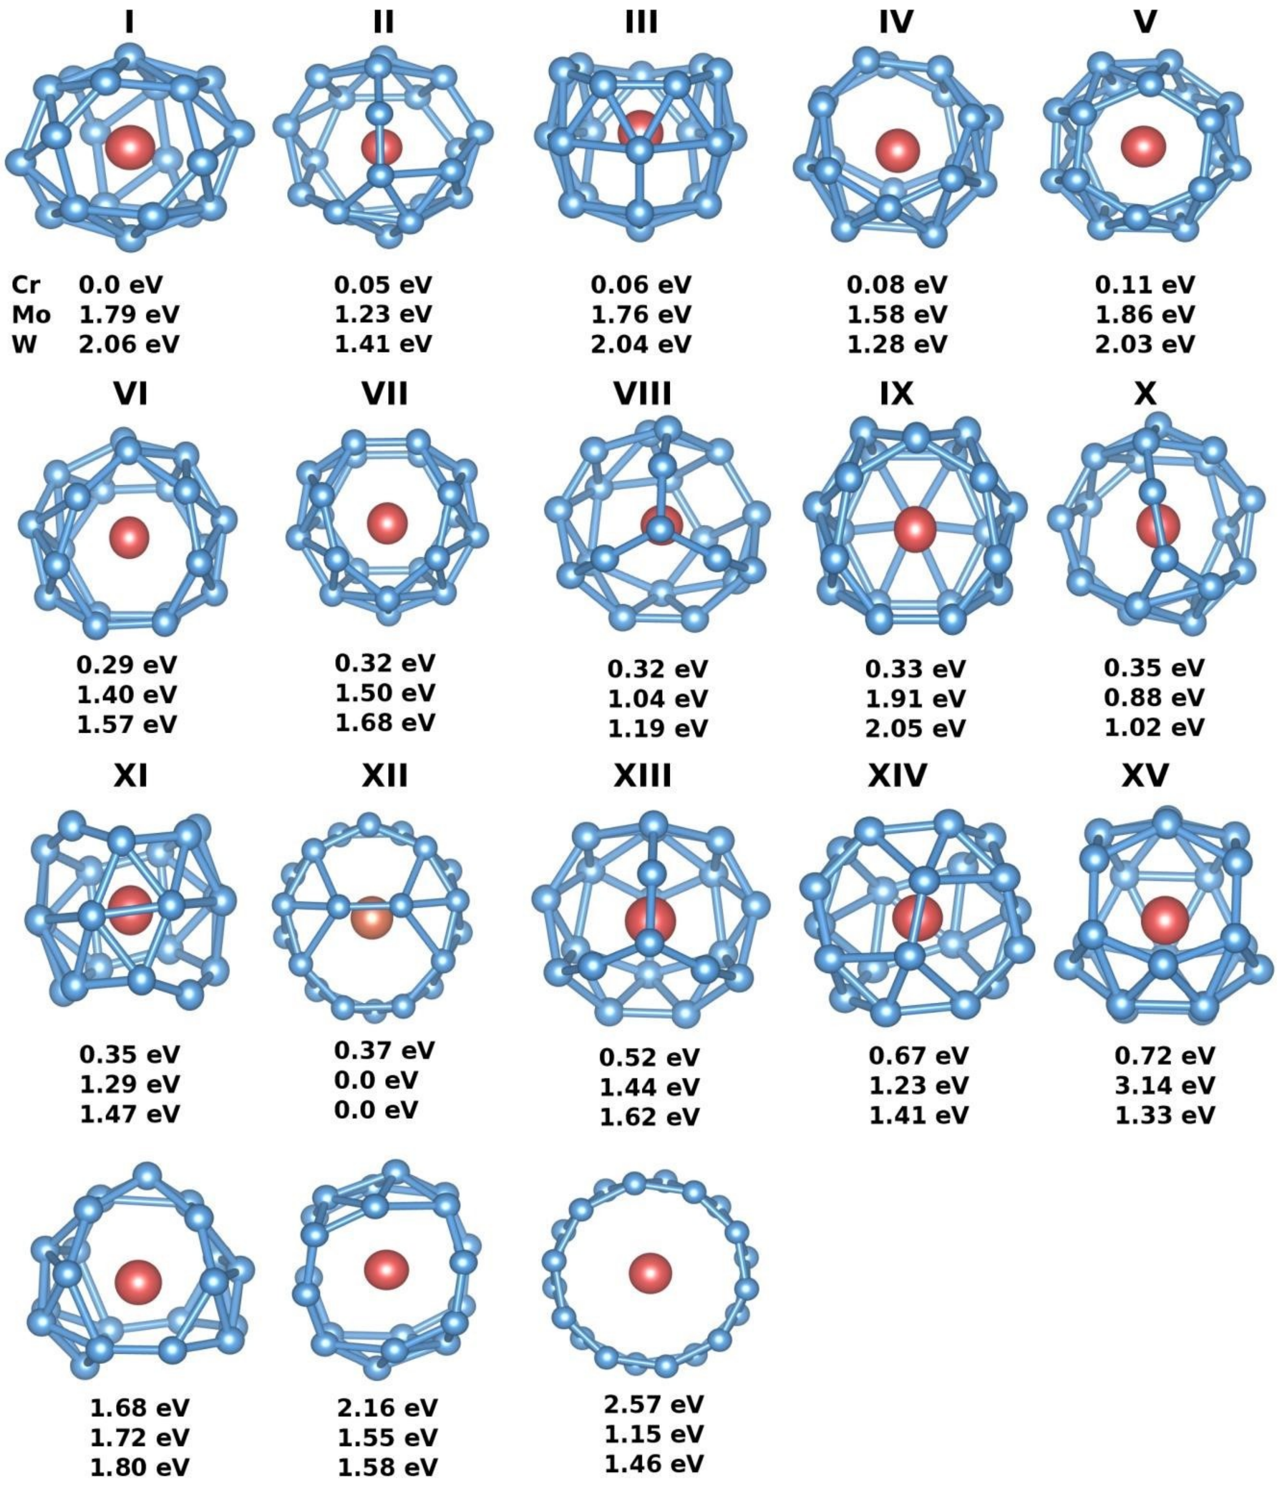


Fig. S2. Same as in Fig. S1 but for $M@B_{20}$ (M = Cr, Mo, and W) using PBE in VASP.

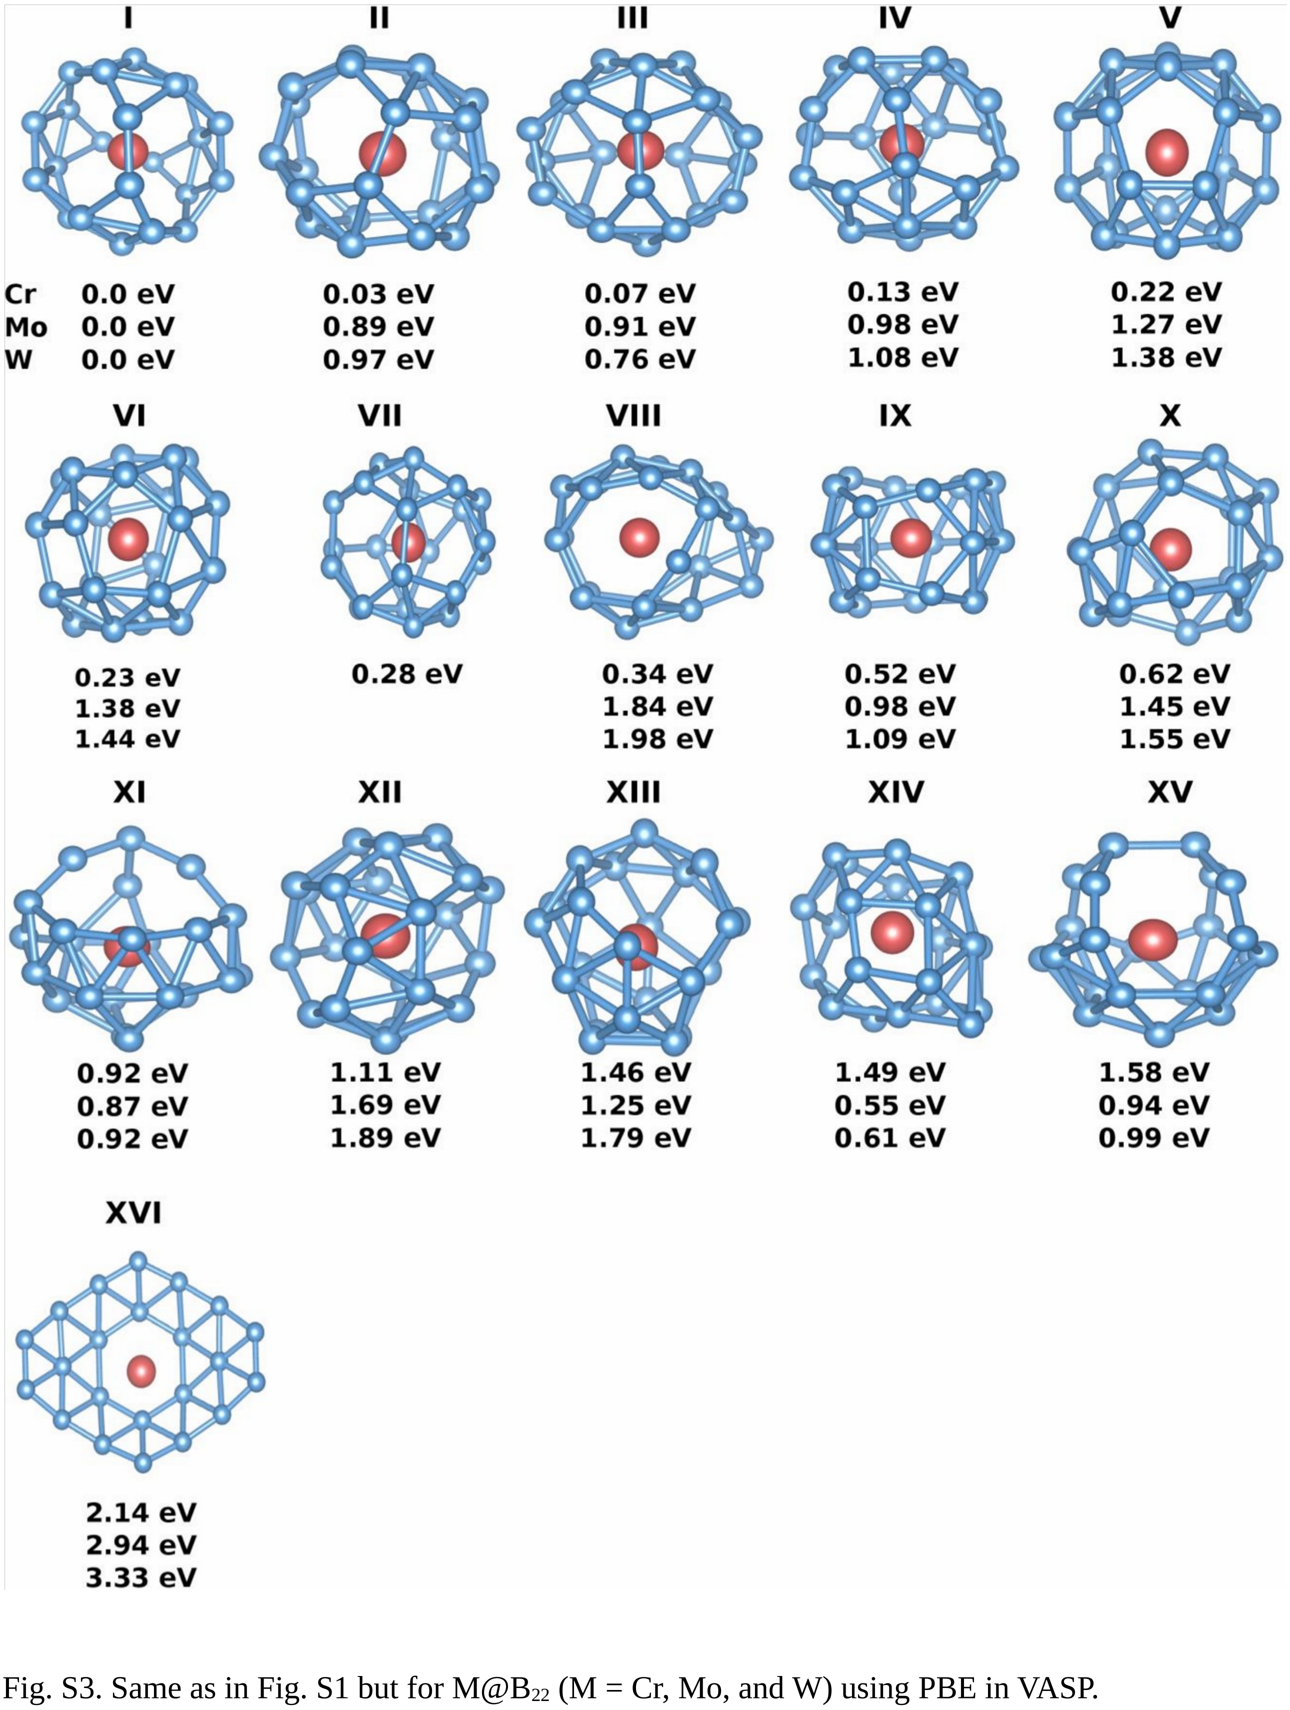


Fig. S3. Same as in Fig. S1 but for $M@B_{22}$ (M = Cr, Mo, and W) using PBE in VASP.

-

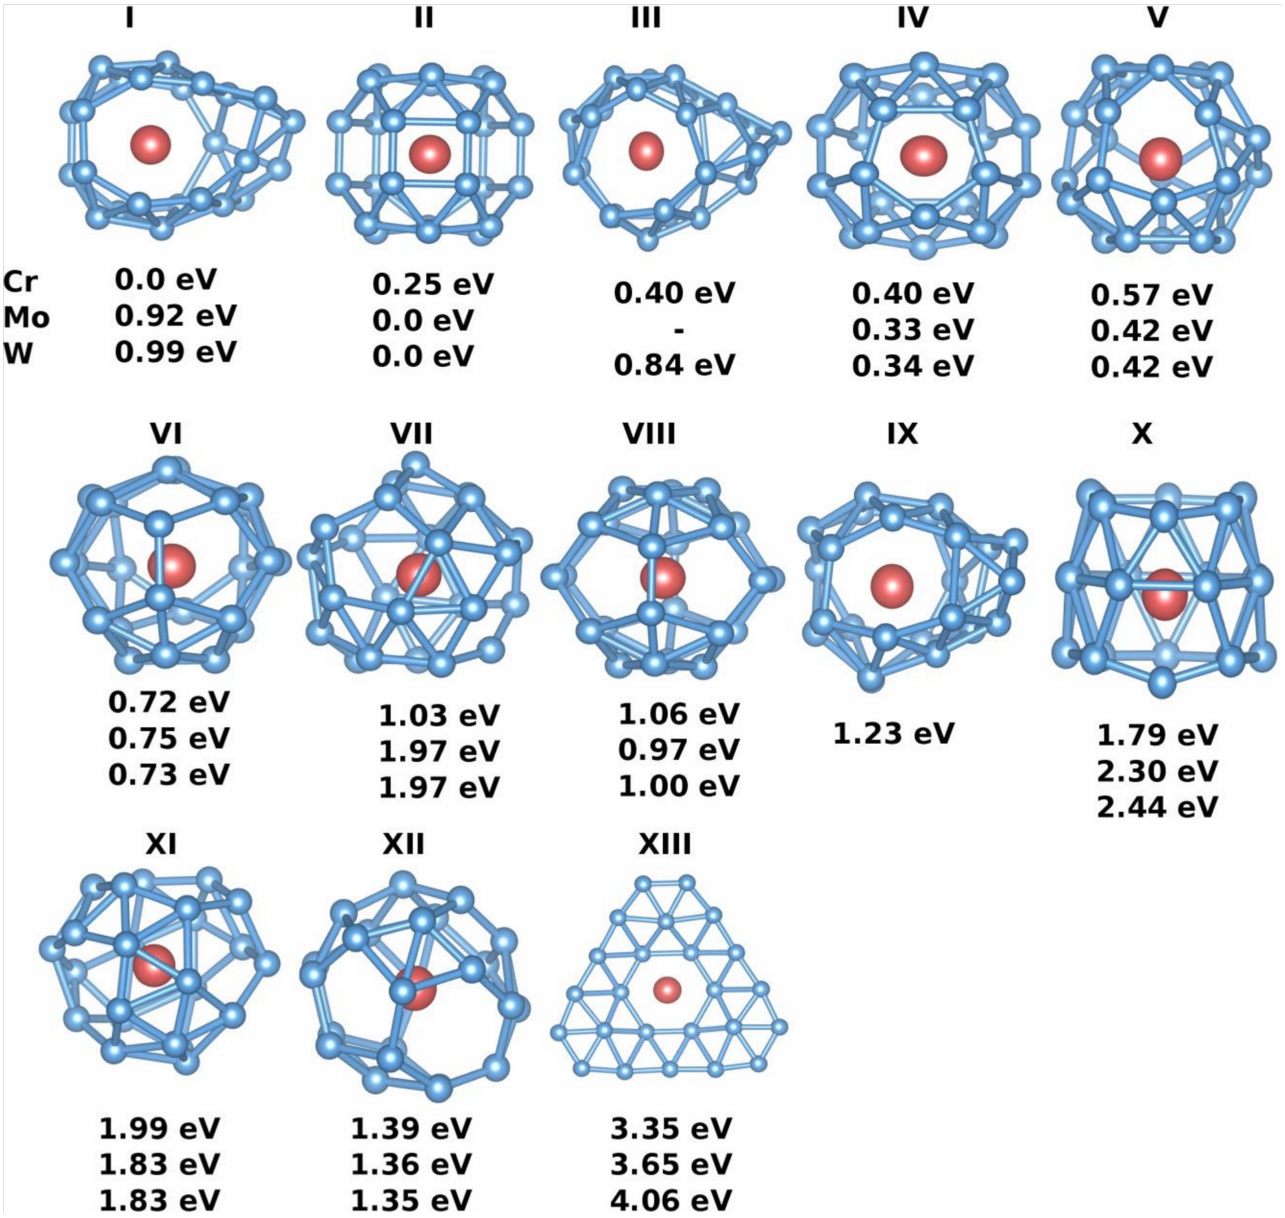


Fig. S4. Same as in Fig. S1 but for $M@B_{24}$ (M = Cr, Mo, and W) using PBE in VASP.

To understand the nature of bonding in these systems we have calculated the total electronic charge density, electron localization function (ELF), and molecular orbitals for some of the cages. Figures S5, S6, and S7 show the total charge density and ELF for the lowest energy structures of $Cr@B_{20}$, $Mo@B_{22}$, and $Mo@B_{24}$, respectively. In some earlier studies multicenter bonding namely 2c, 3c, 4c, 6c, and 7c bonds have been suggested in boron clusters using the AdNDP method to calculate such multi-center two-electron bonds. However, the partitioning in different multi-center bonds with AdNDP method is not unique. We noticed that the shorter B-B bonds (typically ~1.56-1.60 Å) represent 2c-2e bonds, whereas for 3c-2e bonds the bond distances are in the range of 1.60-1.67 Å. The total charge density and ELF surfaces with different iso-values have been helpful in calculating the 2c and multi-center bonds together with the AdNDP analysis.

Figure S5 shows the total charge density and ELF iso-surface plots for the lowest energy isomer of Cr@$B_{20}$. The bond length analysis shows that there are six short B-B bonds with bond distances 1.60 Å. These bonds are along the three 2-member chains joining the three empty heptagons. These bonds are very strong and are detected in the charge density plots at high iso-values as shown in Fig. S5(a), and are also detected from the iso-surfaces of ELF that has six strongly localized lobes as shown in Fig. S5(e). Further decreasing the iso-surface value of the charge density, nine more lobes can be seen in Fig. S5(b), out of which six are placed alternatively on the edges of the two capped hexagons whereas three are placed on the three 2-atom chains. The six lobes are also detected as slightly weaker lobes in the ELF plot as shown in Fig. S5(e). Further decreasing the ELF value, the lobes become larger in size and these represent the six 3c-2e bonds. At slightly lower values of the charge density iso-surface and ELF, the surfaces spread over the entire cluster. We performed similar analysis for metal encapsulated $B_{22}$ and $B_{24}$ cages. Figures S6 and S7 show the total charge density and ELF iso-surfaces for the lowest energy isomers of Mo@$B_{22}$ and Mo@$B_{24}$ endohedral cages, respectively.

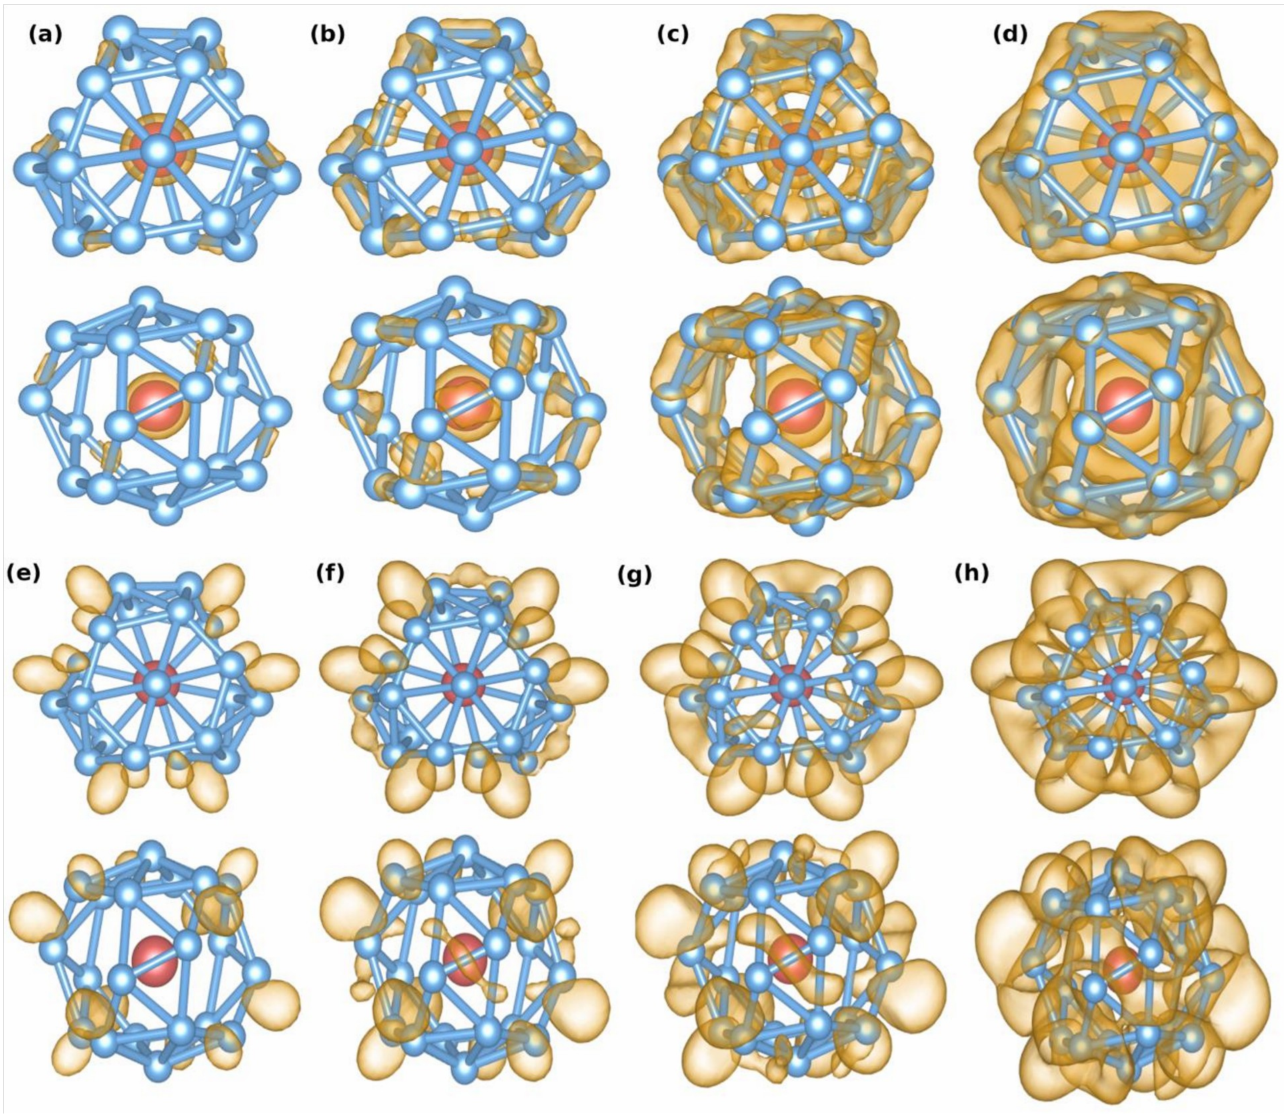


Fig. S5. The total charge density at (a) 27 % (b) 24 % (c) 20 %, and (d) 17 % of the highest value and ELF at (e) 0.88 (f) 0.84 (g) 0.75, and h) 0.70 value of the iso-surface for the lowest energy isomer of $Cr@B_{20}$. The atomic structure is also shown in each case.

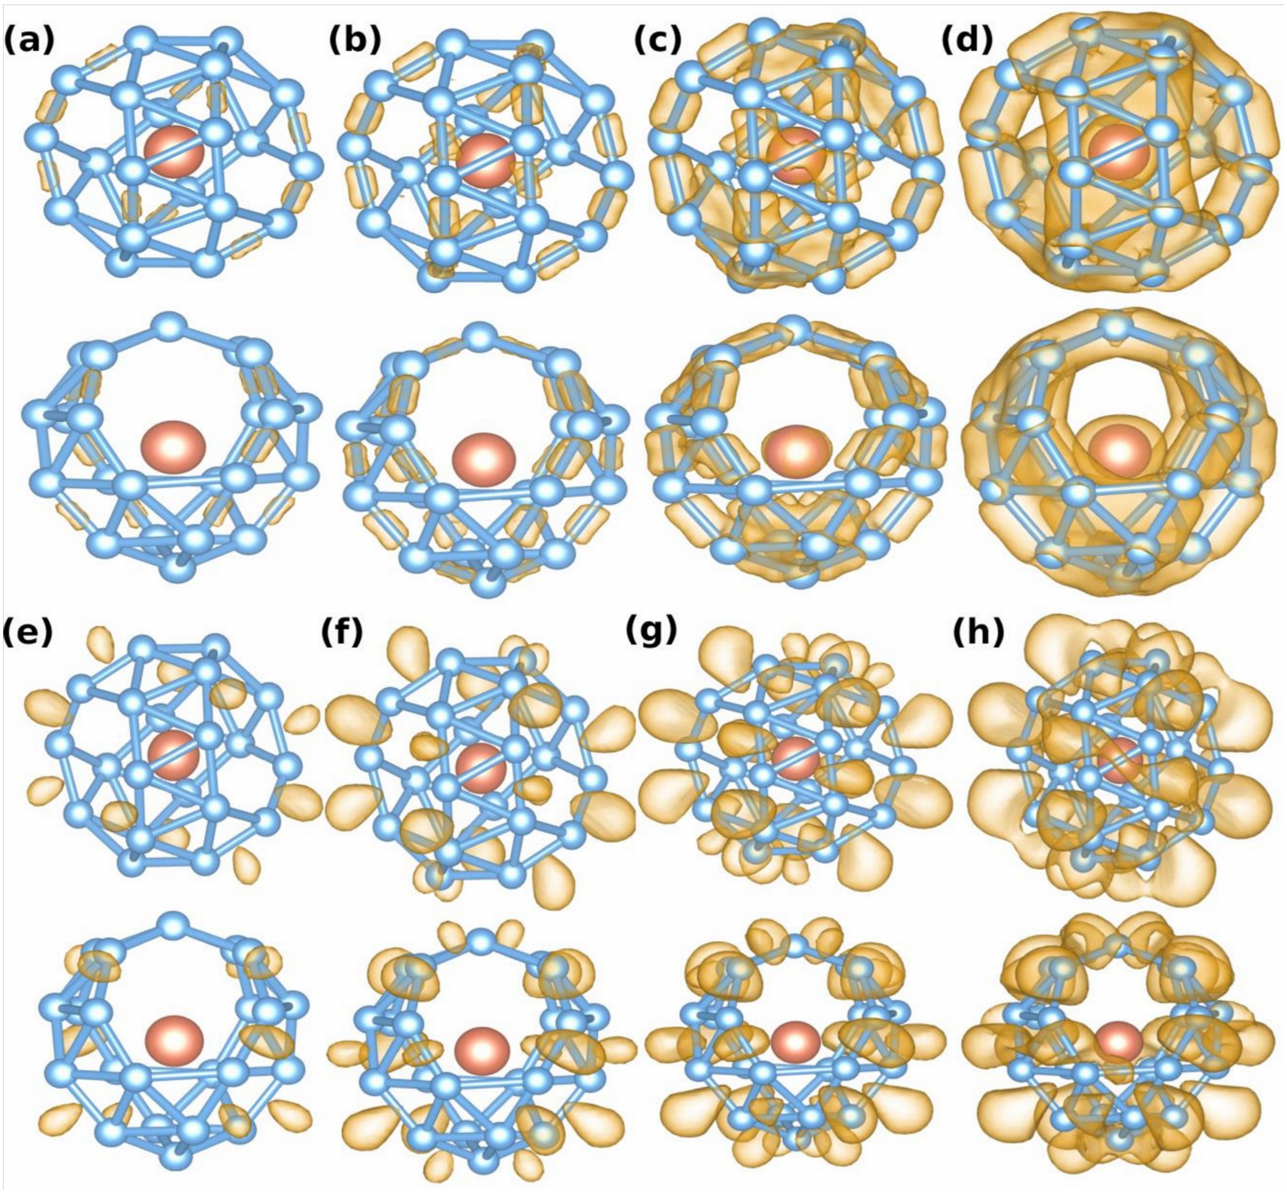


Fig. S6. The total charge density at (a) 80 % (b) 73 % (c) 62.5 %, and (d) 46 % of the highest value and ELF at (e) 0.93 (f) 0.88 (g) 0.82, and (h) 0.76 value of the iso-surface for the lowest energy isomer of Mo@$B_{22}$.

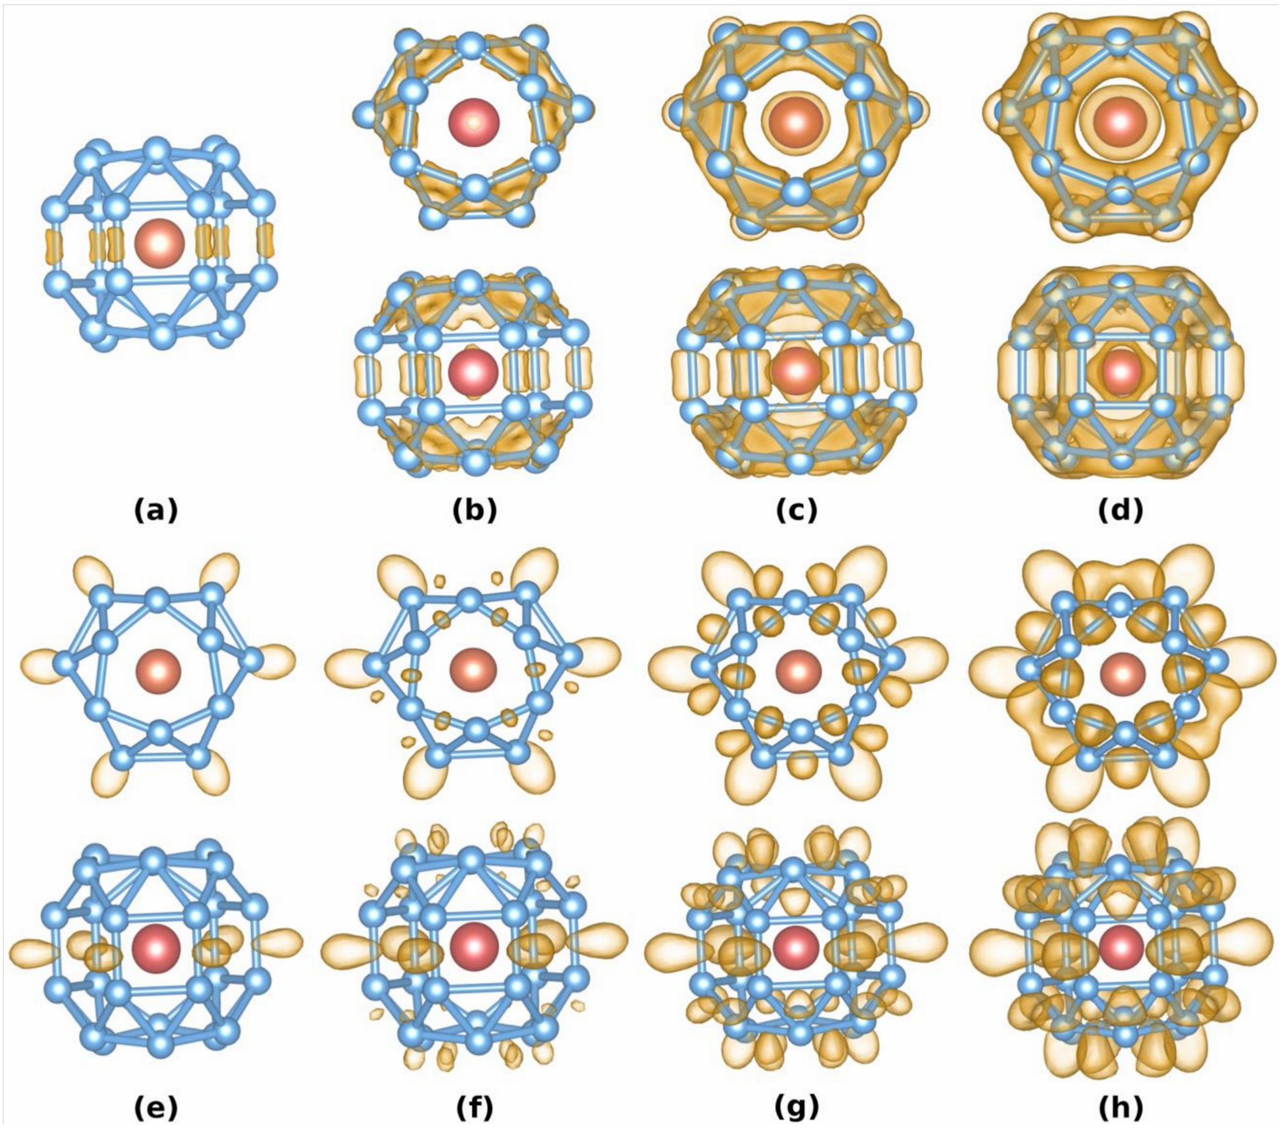


Fig. S7. The total charge density at (a) 76 % (b) 68 % (c) 58 %, and (d) 47 % of the highest value and ELF at (e) 0.92 (f) 0.90 (g) 0.85, and (h) 0.80 value the iso-surface for the lowest energy isomer of Mo@$B_{24}$.

We have shown the Gaussian broadened density of states (DOS) for the anionic clusters corresponding to the neutrals in Figs. S8 while the IR and Raman spectra for the cation clusters are given in Figs. S9. These results will be useful to compare with the experimental results that may become available in future. The major IR and Raman active modes are also listed in Tables S1 and S4. The Cartesian coordinates (in Å) of the lowest energy isomers are given in Tables S5-S11.

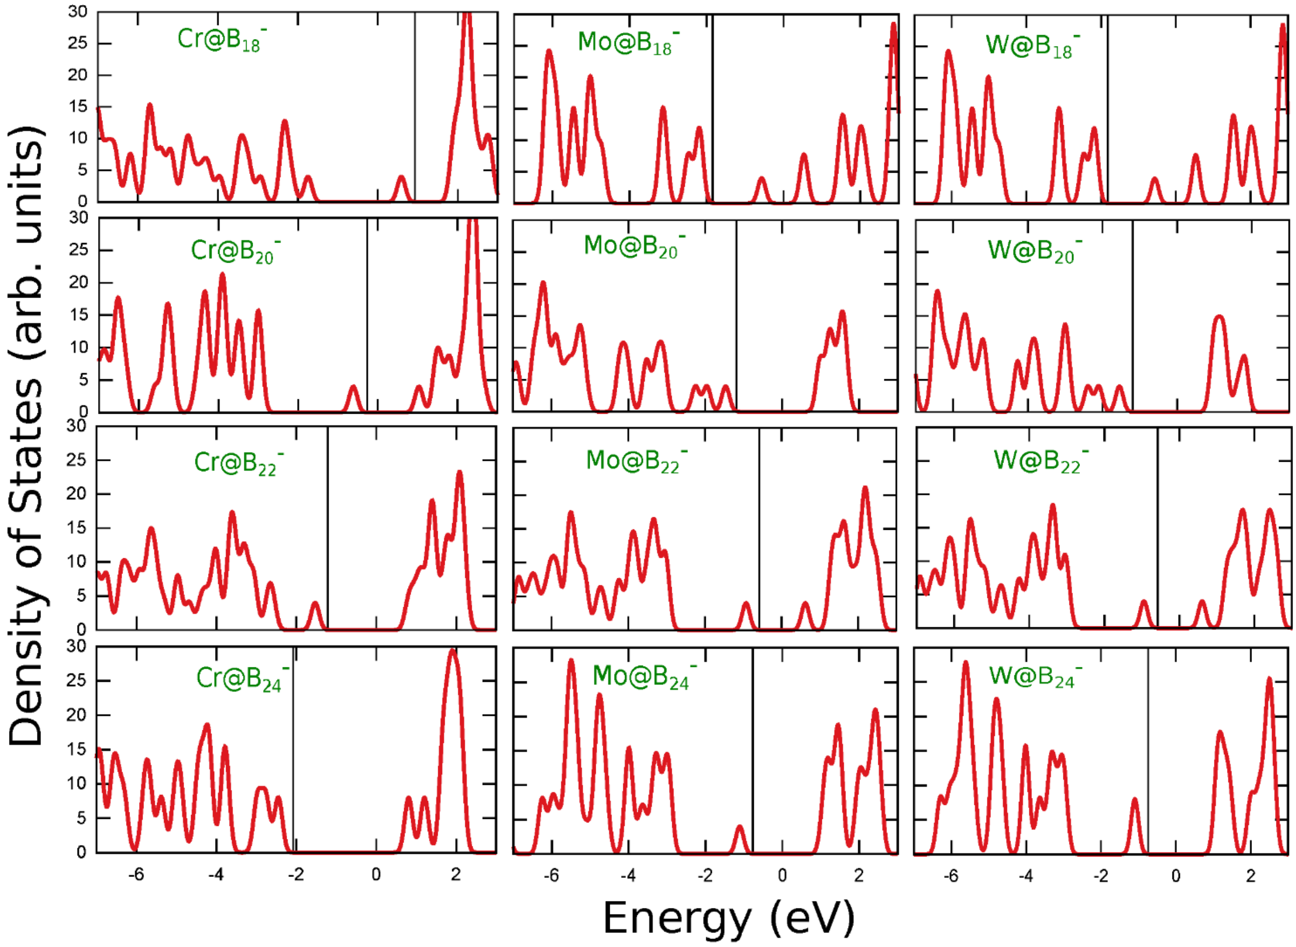


Fig. S8. Calculated Gaussian broadened electronic spectra for the anions of the lowest energy neutral $M@B_{18}$ to $M@B_{24}$ (M = Cr, Mo, and W) clusters. The vertical line shows the HOMO. The spectra have been calculated using Gaussian09 code at the PBE0 level.

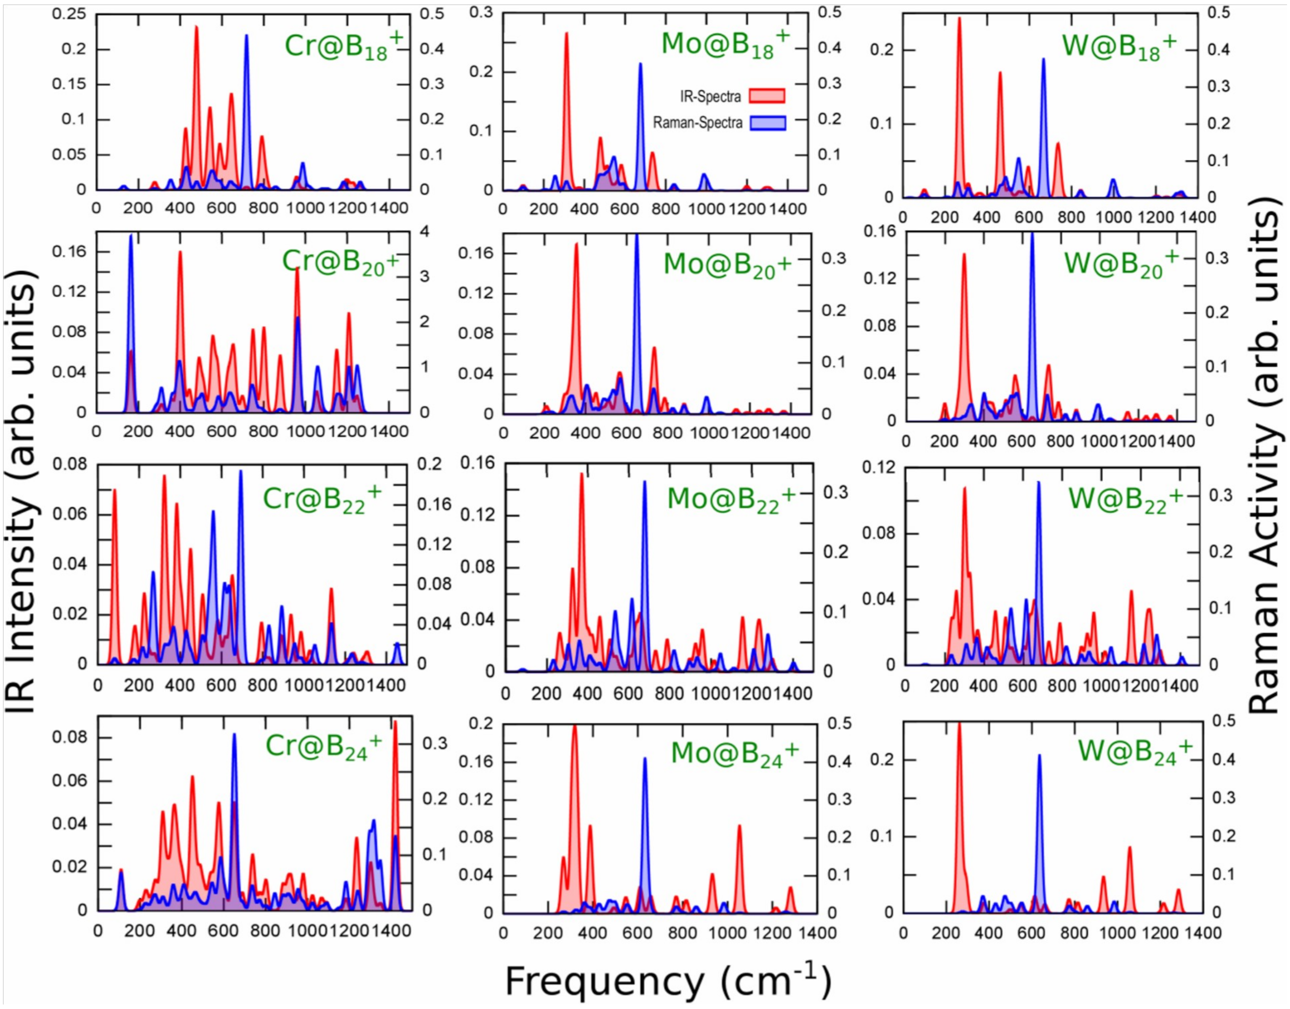


Fig. S9. Calculated IR and Raman spectra of the cations of the lowest energy neutral isomers of $MB_{18}$ to $M@B_{24}$ clusters (M = Cr, Mo, and W). The labels represent the corresponding neutral isomer in Figures S1-S4. The spectra have been calculated using Gaussian09 code at the PBE0 level.

Table S1: Calculated bond distances and vibrational modes using Gaussian G09 code at the B3PW91 level for the lowest energy isomers for neutral $Cr@B_{20}$, $Cr@B_{22}$, $Mo@B_{22}$, $W@B_{22}$, $Mo@B_{24}$, and $W@B_{24}$ clusters. The dominant peaks are marked with asterisk.

| Cluster | Bond lengths (Å) | Vibrational modes ($cm^{-1}$) | | |
|---|---|---|---|---|
| | B-B | B-M | IR intensity (KM/ Mole) | Raman activity (Å$^4$/AMU) |
| $Cr@B_{20}$ | 1.60- 1.83 | 2.08- 2.30 | 388, 433*, 434*, 447, 477*, 481*, 494*, 560, 648*, 651*, 783, 1179, 1190, 1235 | 447, 563, 577, 579, 607, 737*, 772, 777 |
| $Cr@B_{22}$ | 1.56- | 2.31- | 248, 302, 327, | 224, 247, 276*, |

| | | | | |
|---|---|---|---|---|
| | 1.81 | 2.54 | 328, 346, 356*, 372*, 385*, 398, 453, 540, 582, 610, 653, 793, 939, 1155 | 284, 374, 433, 369, 514, 535, 547*, 567, 607*, 633*, 689*, 832, 953, 1068, 1146, 1407 |
| $Mo@B_{22}$ | 1.57-1.84 | 2.38-2.59 | 250, 298, 325*, 331, 349, 370, 375*, 429, 469, 537, 580, 879, 922, 1113, 1289 | 287, 299, 366, 397, 487, 495, 527, 643*, 767*, 888 |
| $W@B_{22}$ | 1.57-1.84 | 2.38-2.59 | 229*, 262*, 282*, 337, 367, 428, 462, 533, 578, 717, 878, 1113, 1286 | 287, 304, 367, 370, 397, 487, 494, 523, 525, 563*, 643*, 767, 888 |
| $Mo@B_{24}$ | 1.64-1.85 | 2.43-2.55 | 254, 256, 292*, 302* 303*, 361, 362, 566, 567, 631, 632, 782, 887, 890, 1021, 1023 | 361, 362, 392*, 433, 497, 499, 504, 505, 596, 597, 613*, 830, 993, 954 |
| $W@B_{24}$ | 1.64-1.85 | 2.43-2.55 | 245*,246*,248*, 269, 271, 565, 567, 631, 632, 779, 885*, 889*, 1022*, 1024* | 346, 348, 365, 366, 372, 374, 392*, 435, 592, 593, 616*, 827, 951, 952 |

Table S2: Calculated vibrational modes using Gaussian G09 at the B3PW91 level for the lowest energy isomers of $Cr@B_{20}^+$, $Cr@B_{22}^+$, $Mo@B_{22}^+$, $W@B_{22}^+$, $Mo@B_{24}^+$, and $W@B_{24}^+$ clusters. The dominant peaks are marked with asterisk.

| Cluster | Vibrational modes ($cm^{-1}$) | |
|---|---|---|
| | IR intensity (KM/Mole) | Raman activity ($Å^4$/AMU) |
| $Cr@B_{20+}$ | 154*, 386, 388*, 394*, 432, 474, 532*, 564, 621, 642, 740*, 779, 877, 956*, 959, 1046, 1135*, 1190* | 154*, 386, 734, 955, 959, 1046, 1062, 1190, 1240 |
| $Cr@B_{22+}$ | 86*, 232*, 288*, 311*, 336, 368*, 407, 506, 529, 617, 647, 649, 790, 941*, 980,1047, 1233, 1298 | 273, 439, 539*, 589, 617,619*, 694*, 831, 910, 942, 1051, 1124, 1412 |
| $Mo@B_{22+}$ | 139, 249, 318*, 326, 340, 345, 356, | 289, 551, 646*, 770, 886, 1022, 1084, |

| | | |
|---|---|---|
| | 368*, 375, 385, 424, 574, 614*, 636*, 693, 722, 873*, 921*, 1024, 1213, 1236, 1273 | 1236, 1257 |
| W@$B_{22}^{+}$ | 133, 225, 238, 257, 268*, 288, 290, | 294, 358, 471, 550, 647*, 784, 889, |
| | 512, 569, 636, 690, 691, 720, 871, 923, 1122, 1216, 1234, 1271 | 1023, 1189, 1234,1260 |
| Mo@$B_{24}^{+}$ | 291*, 293*, 315*, 449, 352*, 546, 631, 658, 664, 772, 992 | 350, 380, 581, 614*, 808, 950 |
| W@$B_{24}^{+}$ | 197, 222, 244*, 256*, 258*, 335, 544, 634, 661, 769, 992 | 353, 380, 578, 615*, 806, 657, 943, 948 |

Table S3: Calculated bond distances and vibrational modes (IR intensity and Raman activity) for the lowest energy isomers for neutral M@$B_{18}$ - M@$B_{24}$ (M = Cr, Mo, and W) clusters using Gaussian09 code at the PBE0 level.

| Cluster | Bond lengths (Å) | Vibrational modes ($cm^{-1}$) | | |
|---|---|---|---|---|
| | B-B | B-M | IR intensity (KM/ Mole) | Raman activity ($Å^4$/AMU) |
| Cr@$B_{18}$ | 1.61- 1.85 | 2.12- 2.36 | 424,476*, 637,788, 983 | 427, 550, 706*, 1022 |
| Mo@$B_{18}$ | 1.58- 1.80 | 2.32- 2.63 | 291*, 298, 210, 220, 466*, 1317 | 334, 515, 591, 611, 620, 675*, 1347 |
| W@$B_{18}$ | 1.58- 1.83 | 2.33- 2.60 | 250*, 268, 455*, 622, 1248, 1330* | 329, 513, 616* ,665* ,1369 |
| Cr@$B_{20}$ | 1.60- 1.83 | 2.08- 2.30 | 455*, 483*, 507, 577, 661, 807, 1196 | 457, 591, 743*, 989 |
| Mo@$B_{20}$ | 1.59- 1.89 | 2.13- 2.57 | 299,355*, 576, 764 | 359, 402, 489, 555, 633*, 762*, 858, 1005 |
| W@$B_{20}$ | 1.57- 1.89 | 2.14- 2.58 | 298*, 347, 576, 635, 755 | 371, 404, 486, 554, 635*, 752, 855, 1005 |
| Cr@$B_{22}$ | 1.56- 1.81 | 2.31- 2.54 | 295,339,388*, 611, 796, 939, 1161, 1341 | 274, 343, 608*, 641*, 702*, 831, 962, 1077, 1160, 1428 |
| Mo@$B_{22}$ | 1.57- 1.84 | 2.38- 2.59 | 317,363*, 389, 414, 542, 646, 780, 927, 1134, | 319, 445, 544, 631*, 675*, 616, 930 |

| | | | | |
|---|---|---|---|---|
| | | | 1305, 1376 | |
| $W@B_{22}$ | 1.57-1.84 | 2.38-2.59 | 272*, 310*, 540, 645, 781, 928, 1135, 1305 | 319, 424, 446, 540, 589, 631*, 676*, 814, 931 |
| $Mo@B_{24}$ | 1.64-1.85 | 2.43-2.55 | 269,324*, 387, 611, 932, 1054, 1281 | 362, 427, 473, 498, 553, 632*, 772, 860, 983, 1259 |
| $W@B_{24}$ | 1.64-1.85 | 2.43-2.55 | 262*, 291, 614, 934, 1058*, 1285 | 371, 430, 473, 552, 635*, 774, 859, 984, 1262 |

Table S4: Calculated vibrational modes (IR intensity and Raman activity) using Gaussian09 code at the PBE0 level for the lowest energy isomers of $Cr@B_{20}^{+}$, $Cr@B_{22}^{+}$, $Mo@B_{22}^{+}$, $W@B_{22}^{+}$, $Mo@B_{24}^{+}$, and $W@B_{24}^{+}$ clusters. The dominant peaks are marked with asterisk.

| Cluster | Vibrational modes ($cm^{-1}$) | |
|---|---|---|
| | IR intensity (KM/Mole) | Raman activity ($Å^4$/AMU) |
| $Cr@B_{18}^{+}$ | 426, 478*, 542, 588, 644, 789 | 429, 553, 716*, 956, 986, 1181, 1261 |
| $Mo@B_{18}^{+}$ | 312*, 479, 581,734 | 509, 547, 676*, 841, 986 |
| $W@B_{18}^{+}$ | 269*, 462, 595, 735 | 487, 549, 667*, 996 |
| $Cr@B_{20}^{+}$ | 163, 401*, 490, 556, 655, 748, 801, 880, 961*, 1150, 1208* | 298, 356*, 403, 450, 568, 736*, 786, 879 |
| $Mo@B_{20}^{+}$ | 298, 356*, 403, 450, 567*, 736 | 406, 535, 570, 650*, 732, 990 |
| $W@B_{20}^{+}$ | 299*, 560, 736, 785 | 337, 401, 541, 571, 651*, 728, 992 |
| $Cr@B_{22}^{+}$ | 81*, 225, 323*, 382*, 450*, 508, 651, 794, 937, 984, 1134 | 268, 560, 637, 694*, 830, 892, 1134, 1153 |
| $Mo@B_{22}^{+}$ | 325, 370*, 458, 634, 655, 958, 1154, 1235 | 359, 533, 614, 678*, 1145, 1208, 1277 |
| $W@B_{22}^{+}$ | 234, 258*, 301, 328*, 457, 508, 655, 785, 958, 1149, 1244 | 536, 614, 678*, 818, 934, 1046, 1213, 1279, 1407 |
| $Mo@B_{24}^{+}$ | 312, 369*, 646, 855, 1031 | 255, 310, 354, 398, 516, 571, 636*, 748, 985 |
| $W@B_{24}^{+}$ | 265*, 297*, 349, 648, 853, 888, 1034 | 257, 349, 403, 516, 543, 570, 638*, 750, 852, 985 |

Table S5: Cartesian coordinates for the isomer I of $Cr@B_{18}$ in Fig. S1.

--------------------------------------------------------------------------------------

19

| | | | |
|---|---|---|---|
| B | 0.7428028158 | 1.4776412362 | 1.3854565363 |
| B | 0.7088349472 | 0.0368653896 | 2.1161608227 |
| B | 0.7335577586 | -1.4302908594 | 1.4393504545 |
| B | 0.5497098193 | 2.2152339619 | -0.0506634191 |
| B | 0.6327216069 | -0.0415448563 | -2.1401430804 |
| B | 0.5355444348 | -2.2190875694 | 0.0313707477 |
| B | 0.6918778936 | 1.4253343040 | -1.4647805707 |
| B | 0.6825007725 | -1.4826970512 | -1.4108943042 |
| B | -0.8287984653 | 0.8631751192 | 2.0572381734 |
| B | -0.8340659376 | -0.7815097297 | 2.0879465821 |
| B | -0.9541871825 | -1.8363441575 | 0.8752695505 |
| B | -0.9839828031 | -1.8661033822 | -0.7718330186 |
| B | -0.9427780335 | 1.8728792647 | 0.8061150976 |
| B | -0.9718192541 | 1.8431709035 | -0.8409688176 |
| B | -0.9023145775 | 0.7876447005 | -2.0569187602 |
| B | -0.9075871362 | -0.8569791254 | -2.0261958528 |
| B | 1.6616166662 | -0.0207355035 | -0.8481353702 |
| B | 1.6908206748 | 0.0087441652 | 0.7884370292 |
| Cr | -0.2711915637 | 0.0009569876 | 0.0048207481 |

--------------------------------------------------------------------------------------

Table S6: Cartesian coordinates for the isomer II of Mo,W@$B_{18}$ in Fig. S1.

--------------------------------------------------------------------------------------

19

| | | | |
|---|---|---|---|
| B | 2.1759790213 | -0.0555604919 | -0.8885590216 |
| B | 1.6066170423 | 1.4551318406 | -0.8852287947 |
| B | -1.2383061305 | 2.1668288412 | -0.7609888871 |
| B | -2.1503492930 | 0.8690833886 | -0.8425280833 |
| B | -1.0625841271 | -2.0405378837 | -0.8633655033 |
| B | 0.4704860167 | -2.4410321995 | -0.7856606422 |
| B | 1.1813016832 | 2.0364439814 | 0.7532045401 |
| B | -0.3941797993 | 2.2336199759 | 0.8241876850 |
| B | -2.3883882425 | -0.0213978181 | 0.6893344542 |
| B | -1.8257203764 | -1.5458587639 | 0.6791009844 |
| B | 1.1537120755 | -1.9590813928 | 0.8032211433 |
| B | 2.2221734475 | -0.7818614936 | 0.7426530613 |
| B | 0.3523148586 | 2.4099825851 | -0.7740577566 |
| B | -1.9573703124 | -0.7150272605 | -0.9419350815 |
| B | 1.8419229431 | -1.5963373025 | -0.7917086696 |
| B | -0.4229842091 | -2.2828301254 | 0.7635092865 |
| B | 2.2417127541 | 0.8255556894 | 0.7037721071 |
| B | -1.8008802142 | 1.4482835404 | 0.7870309792 |
| Mo | -0.0006148808 | -0.0006090187 | 0.0887896261 |

--------------------------------------------------------------------------------------

Table S7: Cartesian coordinates for the isomer I of Cr@$B_{20}$ in Fig. S2.

--------------------------------------------------------------------------------------

21

| | | | |
|---|---|---|---|
| B | 0.4392421684 | -0.6146292501 | 2.1543079644 |
| B | 0.8643021684 | -2.1322492501 | -0.0500320356 |
| B | 0.1058521684 | 2.0475407499 | 1.0035779644 |
| B | -1.8054678316 | -1.1742992501 | 0.2545979644 |

| | | | |
|---|---|---|---|
| B | -1.1221178316 | -0.7821692501 | 1.8506779644 |
| B | -0.2300078316 | 2.2229207499 | -0.5503020356 |
| B | -2.2004178316 | 0.3634607499 | -0.4873420356 |
| B | -0.6820078316 | -2.1297492501 | -0.4586320356 |
| B | -1.1325378316 | 1.0412207499 | -1.5285620356 |
| B | -1.2631378316 | -0.7859292501 | -1.4532920356 |
| B | 0.4555921684 | -1.4117492501 | -1.5819720356 |
| B | 0.0770621684 | 0.0204807499 | -2.2814720356 |
| B | 1.3725121684 | 1.6725207499 | -0.1481820356 |
| B | -0.5056578316 | 0.8445807499 | 1.9324579644 |
| B | 1.2631021684 | 0.7862307499 | 1.4531579644 |
| B | 1.9282721684 | -1.0824792501 | -0.6380220356 |
| B | 2.2601021684 | 0.3129107499 | 0.0695779644 |
| B | 1.6155621684 | -0.9721992501 | 1.0716379644 |
| B | -1.9941178316 | 0.3373807499 | 1.0984879644 |
| B | 0.5537621684 | 1.4364907499 | -1.7109020356 |
| Cr | 0.0000221684 | -0.0000592501 | 0.0000479644 |

---------------------------------------------------------------------------------------

Table S8: Cartesian coordinates for the isomer XII of Mo@$B_{20}$ in Fig. S2.

---------------------------------------------------------------------------------------

21

| | | | |
|---|---|---|---|
| B | 2.3305543570 | -0.0024093919 | -0.8634027510 |
| B | 1.8180604478 | 1.5133337295 | -0.8546430004 |
| B | -1.1739911886 | 1.9955885600 | -0.9086011573 |
| B | -2.2219213232 | 0.7878486342 | -0.8767760041 |
| B | -1.1543477160 | -2.0318043077 | -0.9801258979 |
| B | 0.4273245077 | -2.3487353108 | -1.0049356295 |
| B | 1.1244765732 | 1.9706376017 | 0.7973006582 |
| B | -0.4236152730 | 2.3375785620 | 0.6961438807 |
| B | -2.2995356925 | -0.0420281261 | 0.7851402811 |
| B | -1.6315380091 | -1.4869248457 | 0.8012390466 |
| B | 1.1787677063 | -2.1384961095 | 0.5943979978 |
| B | 2.0382423842 | -0.8277760201 | 0.8215694348 |
| B | 0.4157644042 | 2.2810517061 | -0.8999506678 |
| B | -2.1746950788 | -0.8114972543 | -0.8882158424 |
| B | 1.7994838846 | -1.5012838377 | -0.9639293562 |
| B | -0.3672964842 | -2.4162609125 | 0.5858695042 |
| B | 2.1620280856 | 0.7593257049 | 0.8095845254 |
| B | -1.7482988954 | 1.4547129192 | 0.7815435624 |
| B | -0.8569328083 | 0.1064089030 | 1.7245824151 |
| B | 0.7482592741 | 0.3942378983 | 1.7334102227 |
| Mo | 0.0010378281 | 0.0007314719 | -0.2129776445 |

---------------------------------------------------------------------------------------------------

Table S9: Cartesian coordinates for the isomer I of M@$B_{22}$ (Cr, Mo, W) in Fig. S3.

---------------------------------------------------------------------------------------------------

23

| | | | |
|---|---|---|---|
| B | 0.0646915385 | -0.7812792713 | 2.3667091095 |
| B | -1.4440584615 | -0.4970092713 | 1.9821891095 |
| B | 1.3999415385 | -1.2226492713 | 1.6615691095 |
| B | -0.1668484615 | -2.4016292713 | -0.4865608905 |

| | | | |
|---|---|---|---|
| B | 0.5083515385 | 1.9345707287 | 1.4252091095 |
| B | -0.5622384615 | 0.9282307287 | 2.1183991095 |
| B | -2.3608784615 | -0.6365992713 | 0.5416691095 |
| B | -1.6455484615 | -1.8355692713 | -0.3063008905 |
| B | 1.3277015385 | -1.9753692713 | -0.0134208905 |
| B | 2.3425115385 | -0.7321692713 | 0.4884391095 |
| B | -1.0822884615 | 2.0647107287 | 0.7733891095 |
| B | -2.1688784615 | -0.4776292713 | -1.1533508905 |
| B | -0.8559184615 | -1.3108092713 | -1.7929408905 |
| B | 0.7411415385 | -1.5978192713 | -1.7118308905 |
| B | 2.3608015385 | 0.6366607287 | -0.5417208905 |
| B | 1.6500015385 | 1.8295807287 | 0.3184791095 |
| B | -0.1756784615 | 1.5529707287 | -1.9422608905 |
| B | 0.0905415385 | 2.3579707287 | -0.3119308905 |
| B | -1.2892284615 | 0.4509607287 | -2.0855808905 |
| B | 1.2704015385 | 1.7065407287 | -1.3174408905 |
| B | 2.0292915385 | -0.8371692713 | -1.1628708905 |
| B | -2.0336484615 | 0.8433207287 | 1.1506991095 |
| Mo | -0.0000184615 | 0.0000207287 | -0.0000608905 |

------------------------------------------------------------------------------------------

Table S10: Cartesian coordinates for the isomer III of Cr@$B_{22}$ in Fig. S3.

------------------------------------------------------------------------------------------

23

| | | | |
|---|---|---|---|
| B | 2.3399305051 | -0.0356224800 | -0.4755702032 |
| B | 1.7951535051 | 1.5090965200 | -0.5100002032 |
| B | -1.1320804949 | 1.8709325200 | -1.0083922032 |
| B | -2.0712604949 | 0.5846115200 | -0.7622582032 |
| B | -1.1402324949 | -1.8590874800 | -1.1454082032 |
| B | 0.4005875051 | -2.2192924800 | -0.9932782032 |
| B | 0.9855035051 | 1.9103975200 | 1.1454797968 |
| B | -0.3165114949 | 2.4216445200 | 0.3515437968 |
| B | -2.0771644949 | 0.1137495200 | 0.9948047968 |
| B | -1.4590044949 | -1.3646744800 | 1.3678417968 |
| B | 1.2120105051 | -2.0098884800 | 0.4526737968 |
| B | 1.8486455051 | -0.7742674800 | 1.2534767968 |
| B | 0.4423175051 | 1.9176115200 | -1.3151142032 |
| B | -2.1797314949 | -0.9906664800 | -0.2827912032 |
| B | 1.5832215051 | -1.1736654800 | -1.3228392032 |
| B | -0.4134214949 | -2.2993894800 | 0.4796677968 |
| B | 2.1173905051 | 0.7850885200 | 0.9648127968 |
| B | -1.7089374949 | 1.6164215200 | 0.5987457968 |
| B | -0.6295714949 | -0.1996204800 | 2.1505387968 |
| B | 0.8499315051 | 0.4445095200 | 2.0856247968 |
| B | -0.5268404949 | 0.6514455200 | -2.0248272032 |
| B | 0.0171605051 | -0.9137714800 | -2.0744962032 |
| Cr | 0.0130775051 | 0.0030015200 | 0.0145037968 |

------------------------------------------------------------------------------------------

Table S11: Cartesian coordinates for the isomer II of Mo@$B_{24}$ in Fig. S4.

| | | | |
|---|---|---|---|
| B | 1.1402575286 | -1.0498026994 | 1.8771285171 |
| B | -1.0360224714 | 2.0140673006 | 1.1746385171 |
| B | -2.1317924714 | 1.1605273006 | 0.1856185171 |
| B | -2.3851624714 | -0.4628126994 | 0.1510685171 |
| B | -0.6582424714 | -0.7762326994 | 2.2112685171 |
| B | -1.0765124714 | 2.2563573006 | -0.4590114829 |
| B | -1.5132024714 | 1.1011173006 | -1.5566114829 |
| B | -1.7094524714 | -1.8001926994 | -0.5454014829 |
| B | -0.0537924714 | -2.1007126994 | 1.4298485171 |
| B | -0.0212024714 | 1.9168473006 | -1.6836114829 |
| B | -1.6076924714 | -1.6498526994 | 1.0965385171 |
| B | -1.7667124714 | -0.5222426994 | -1.5911414829 |
| B | 0.8136675286 | -2.1838926994 | -1.0142814829 |
| B | -0.5930924714 | -1.7472426994 | -1.7619914829 |
| B | 0.5791675286 | 1.9559173006 | 1.5162785171 |
| B | -0.4050224714 | 0.8471873006 | 2.2458785171 |
| B | 1.3934475286 | 0.5736073006 | 1.9117185171 |
| B | 0.8649075286 | -0.9223626994 | -2.0801314829 |
| B | 1.3431375286 | -2.0987626994 | 0.5482285171 |
| B | 2.0449675286 | -1.1365526994 | -0.6720414829 |
| B | 2.2983675286 | 0.4867573006 | -0.6373614829 |
| B | 1.9149775286 | 1.5652873006 | 0.6264085171 |
| B | 1.4469075286 | 1.8726173006 | -0.9276414829 |
| B | 1.1182075286 | 0.7010173006 | -2.0454714829 |
| Mo | -0.0000124714 | -0.0000726994 | 0.0000085171 |
